# Supplementary material for: Keeping Deep Learning Models in Check: A History-Based Approach to Mitigate Overfitting
Source: arXiv:2401.10359 source file (2024-01-18)
Supplement: Supplementary file 1 [file appendix.tex]

\section{A heuristic approach for automatic labelling}\label{appendix:auto_label}

We developed a heuristic approach for labelling the training history in the simulated dataset as overfitting based on the following conditions:

\begin{itemize}
  \item The training loss and validation loss both decrease in the first $inc_p$ percentage of the training history.
  \item The training loss and validation loss both decrease in the last $dec_p$ percentage of the training history.
  \item The gap between the training loss and validation loss exceeds $gap_p$ percentage of the sum of the training and validation loss.
\end{itemize}

To select the thresholds, we performed a grid search between 10\% to 50\% for $inc_p$ and $dec_p$, and a grid search between 1\% to 50\% for $gap_p$. The best performance of the heuristic approach can achieve is a 0.75 F-score for the overfitting samples with 0.96 precision and 0.61 recall. The result shows that the heuristic approach does not work well on the simulated dataset in comparison to other approaches (see Table~\ref{tab:res_test_set}). Furthermore, the heuristic approach performs poorly on the real-world dataset, with a 0.22 average F-score. Hence, human labels are still required for labelling the data for training the time series classifiers to be used in our approach.

\section{Using zero-one loss for overfitting prevention}\label{appendix:acc_curve}

\begin{table}[tbhp]
\small
\centering
\caption{Results of the average classification accuracy of obtained models in the real-world dataset using overfitting prevention methods based on zero-one validation loss curves. (ES: early stopping; ES-SC: early stopping with smoothed curves; OPT: optimal classification accuracy)}
\label{tab:avg_cls_acc_error}
\begin{tabular}{rrrrrrrrrr}
\toprule
Ws. & BOSSVS & HMM-GMM & KNN-DTW & SAX-VSM & TSBF  & TSF   & ES    & ES-SC & OPT                    \\ \midrule
20  & 0.415  & 0.354   & 0.417   & 0.371   & 0.377 & 0.396 & 0.395 & 0.394 &  \multirow{5}{*}{0.434} \\
40  & 0.428  & 0.374   & 0.431   & 0.375   & 0.387 & 0.401 & 0.426 & 0.426 &                        \\
60  & 0.429  & 0.384   & 0.433   & 0.384   & 0.394 & 0.407 & 0.433 & 0.433 &                        \\
80  & 0.430  & 0.387   & 0.434   & 0.389   & 0.415 & 0.432 & 0.433 & 0.433 &                        \\
100 & 0.431  & 0.406   & 0.434   & 0.394   & 0.424 & 0.434 & 0.433 & 0.434 &                       \\ \bottomrule
\end{tabular}
\end{table}

\begin{table}[tbhp]
\centering
\small
\captionof{table}{The median delay and significant testing of our overfitting prevention methods based on zero-one validation loss curves with different window sizes. (Ws.: Window size; Md.: Median delay)}
\label{tab:stop_delay_epoch_acc}
\begin{tabular}{@{}rlrrrr|lrrrr@{}}
\toprule
Ws. &
  Classifier &
  Md. &
  P &
  \begin{tabular}[c]{@{}r@{}}Effect\\ size\end{tabular} &
  \begin{tabular}[c]{@{}r@{}}Cliff's\\ d value\end{tabular} &
  Classifier &
  Md. &
  P &
  \begin{tabular}[c]{@{}r@{}}Effect\\ size\end{tabular} &
  \begin{tabular}[c]{@{}r@{}}Cliff's\\ d value\end{tabular} \\ \midrule
20  & \multirow{5}{*}{BOSSVS}  & 13.5 & 0.684 & neg    & -0.050 & \multirow{5}{*}{SAX-VSM} & 5.0  & 0.000 & large  & -0.950 \\
40  &                          & 46.0 & 0.109 & small  & 0.198  &                          & 5.5  & 0.000 & large  & -0.976 \\
60  &                          & 44.5 & 0.494 & neg    & -0.087 &                          & 11.5 & 0.000 & large  & -0.884 \\
80  &                          & 46.5 & 0.115 & small  & -0.202 &                          & 14.5 & 0.000 & large  & -0.806 \\
100 &                          & 49.5 & 0.029 & small  & -0.284 &                          & 26.5 & 0.000 & large  & -0.716 \\ \midrule
20  & \multirow{5}{*}{HMM-GMM} & 2.0  & 0.000 & large  & -0.850 & \multirow{5}{*}{TSBF}    & 7.5  & 0.000 & large  & -0.750 \\
40  &                          & 5.0  & 0.000 & large  & -0.739 &                          & 14.5 & 0.000 & large  & -0.867 \\
60  &                          & 8.0  & 0.000 & large  & -0.656 &                          & 27.0 & 0.000 & large  & -0.809 \\
80  &                          & 18.0 & 0.000 & large  & -0.719 &                          & 37.0 & 0.000 & large  & -0.708 \\
100 &                          & 46.5 & 0.001 & medium & -0.431 &                          & 45.0 & 0.000 & large  & -0.561 \\ \midrule
20  & \multirow{5}{*}{KNN-DTW} & 48.5 & 0.000 & large  & 0.650  & \multirow{5}{*}{TSF}     & 12.5 & 0.001 & medium & -0.400 \\
40  &                          & 44.0 & 0.027 & small  & 0.273  &                          & 24.0 & 0.000 & large  & -0.726 \\
60  &                          & 47.0 & 0.392 & neg    & -0.109 &                          & 31.0 & 0.000 & large  & -0.630 \\
80  &                          & 48.5 & 0.194 & small  & -0.166 &                          & 42.5 & 0.000 & large  & -0.596 \\
100 &                          & 56.5 & 0.024 & small  & -0.292 &                          & 47.0 & 0.000 & large  & -0.479 \\ \bottomrule
\end{tabular}
\end{table}

Overfitting prevention methods may stop the training process by inspecting the validation accuracy error (i.e., zero-one loss) rather than the loss utilized for optimizing the model. Figure~\ref{fig:cmp_correct_rate_acc} shows the optimal rate of our approaches as well as early stopping based on zero-one validation loss. When compared to the results in Figure~\ref{fig:cmp_correct_rate} (which uses validation loss), the optimal rate of early stopping based on zero-one loss is quite similar. The results show that the optimal rate improves (with an average of 2.5\%) when the patience value is between 35 and 90 epochs but declines (with an average of 2.9\%) when the patience value is less than 35 epochs. 
For our method with KNN-DTW, the results show that using zero-one loss curves increases the optimal rate, which still outperforms early stopping and other time series classifiers. However, the delay of the KNN-DTW also increases and stops later than early stopping when the window size is less than or equal to 40 epochs (as shown in Table~\ref{tab:stop_delay_epoch_acc}). We found that our approach with KNN-DTW has a higher optimal rate but longer delay while using the zero-one loss curves (compared to using the original loss curves). Furthermore, Table~\ref{tab:avg_cls_acc_error} shows that when using zero-one loss curves, our method with KNN-DTW has higher average accuracy than early stopping.

\begin{figure}[tb]
    \centering
    \includegraphics[width=\columnwidth]{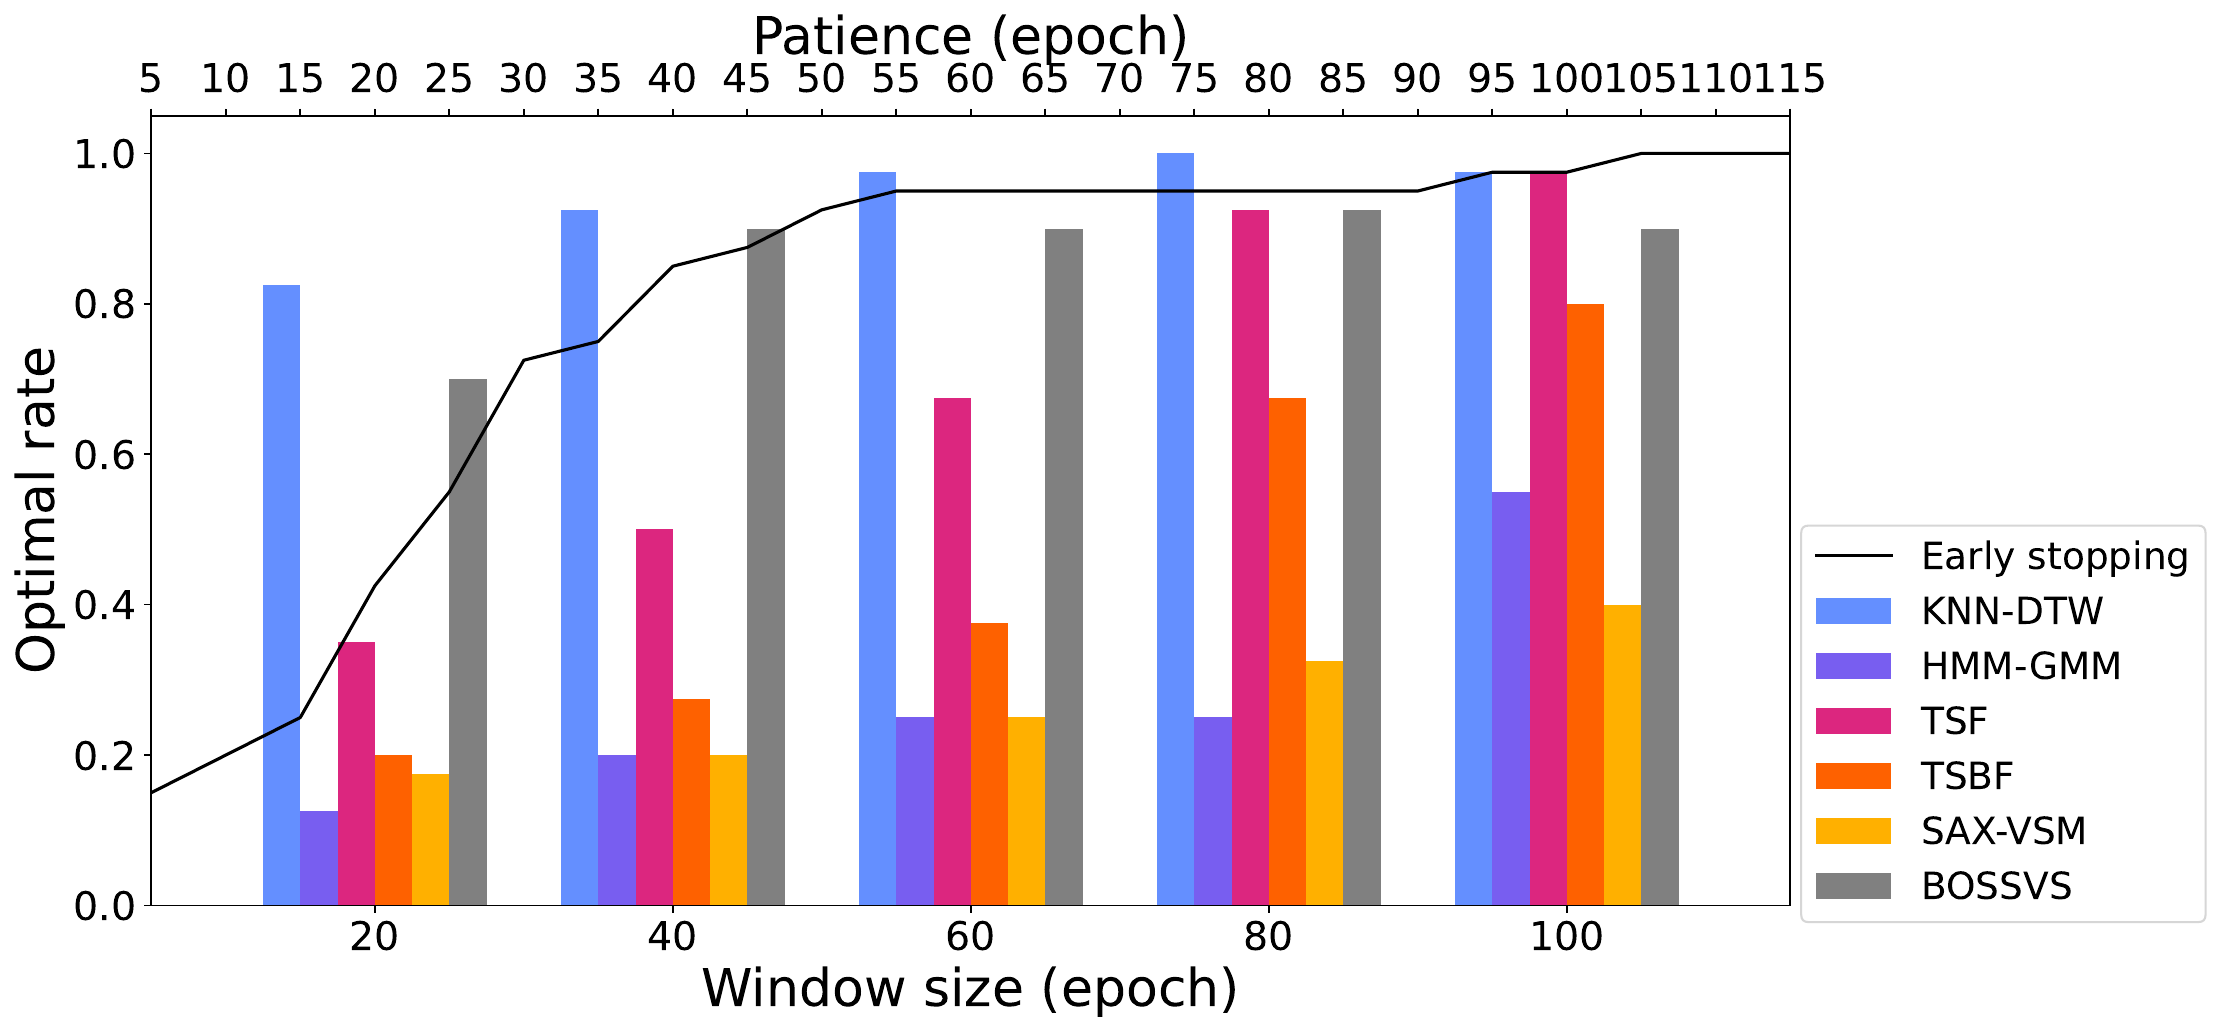}
    \caption{The optimal rate of our approaches~(using a rolling window) and early stopping with different patience values based on zero-one validation loss curves.}
    \label{fig:cmp_correct_rate_acc}
\end{figure}
